# Supplementary material for: Correlation Coefficients and Semantic Textual Similarity
Source: arXiv:1905.07790 source file (2019-05-19)
Supplement: Supplementary file 1 [file appendix.tex]

\onecolumn
\section*{Appendix}

\input{tables/cis.tex}
